# Supplementary material for: The Inductive Bias of Flatness Regularization for Deep Matrix Factorization
Source: arXiv:2306.13239 source file (2023-06-22)
Supplement: Supplementary file 1 [file additional_experiments.tex]

\section{Experiments}
